# Supplementary material for: CProp: Adaptive Learning Rate Scaling from Past Gradient Conformity
Source: arXiv:1912.11493 source file (2019-12-24)
Supplement: Supplementary file 1 [file appendix.tex]

\input{latex/sections/appendix/architectures.tex}
\input{latex/sections/appendix/optimizer.tex}
\input{latex/sections/appendix/dataset.tex}
\input{latex/sections/appendix/alternatives.tex}
\input{latex/sections/appendix/lr_selection.tex}
